# Supplementary material for: Software Verification for Weak Memory via Program Transformation
Source: arXiv:1207.7264 source file (2012-07-30)
Supplement: Supplementary file 1 [file appendix.tex]

% vi: filetype=tex spell spelllang=en_gb:

\section*{Appendix}

\begin{lstlisting}[caption={C source code of token passing}, label={prog:pgsql}]
#define WORKERS 2
volatile _Bool latch[WORKERS];
volatile _Bool flag[WORKERS];

void worker(int i) 
{ 
  while(!latch[i]);
  for(;;) 
  { 
    assert(!latch[i] || flag[i]); (*@ \label{pgsql:starve} @*)
    latch[i] = 0; (*@ \label{pqsql:setlatch} @*)
    if(flag[i]) (*@\label{pgsql:dowork} @*)
    { 
      flag[i] = 0; 
      flag[i+1 % WORKERS] = 1; (*@\label{pgsql:nextflag}@*)
      latch[i+1 % WORKERS] = 1; (*@\label{pgsql:nextlatch}@*)
    } 

    while(!latch[i]); (*@ \label{pgsql:waitlatch} @*)
  } 
}
\end{lstlisting}

\begin{table}[h]
\centering
\begin{tabular}{llcr}
%\toprule
Test    & Cycle                           & Relaxed if $\leq$ & Source Lines \\ \midrule
mix012  & $\rfi~\poi{\textsf{dRR}}~\efr~\poi{\textsf{dWR}}~\efr$         & TSO        & 241, 151, 153, 232 \\
mix034  & $\rfi~\poi{\textsf{dRR}}~\efr~\poi{\textsf{dWR}}~\efr~\poi{\textsf{dWW}}$   & TSO        & 242, 150, 150, 151, 170, 232 \\
rfi001  & $\rfi~\poi{\textsf{dRR}}~\efr~\poi{\textsf{dWW}}~\ews~\poi{\textsf{dWW}}$   & TSO        & 242, 150, 150, 151, 170, 232 \\
rfi007  & $\rfi~\poi{\textsf{dRR}}~\efr~\poi{\textsf{dWW}}~\ews$         & TSO        & 241, 151, 153, 170, 232 \\
safe006 \ltest{(lb)} & $\rfe~\poi{\textsf{dRW}}~\rfe~\poi{\textsf{dRW}}$             & RMO        & 98, 241, 242, 66 \\
safe010 & $\rfe~\poi{\textsf{dRW}}~\ews~\poi{\textsf{dWW}}$             & PSO        & 150, 273, 276, 149 \\
safe012 & $\rfe~\poi{\textsf{dRW}}~\rfe~\poi{\textsf{dRR}}~\efr~\poi{\textsf{dWW}}$   & PSO        & 242, 66, 90, 165, 170, 232 \\
safe022 \ltest{(mp)} & $\rfe~\poi{\textsf{dRR}}~\efr~\poi{\textsf{dWW}}$             & PSO        & 146, 98, 99, 146 \\
%\bottomrule
\end{tabular}
\vspace{1mm}
\caption{Overview of cycles in RCU corresponding to existing litmus tests \label{tab:rcu-cycles}}
\end{table}

\endinput

\section{Detailed Data of Experimental Results}

\begin{table}[h]
\centering
\begin{tabular}{lrrrrr}
\toprule
Category        & \#Tests  &  Spurious  &  Avg.~Time & Avg.~Overhead & Overhead 1d \\ \midrule 
x86/mix         & 58       &  0/0/0/0\\
x86/podwr       & 2        &  0/0/0/0\\
x86/rfi         & 11       &  0/0/0/0\\
x86/safe        & 38       &  0/0/0/1\\
x86/thin        & 3        &  0/0/0/0\\
ppc/cross       & 3        &  0/0/0/0\\
ppc/mix         & 209      &  0/0/0/0\\
ppc/aclwdrr     & 16       &  0/0/0/1\\
ppc/aclwsrr     & 3        &  0/0/0/0\\
ppc/bclwdww     & 10       &  0/0/0/3\\
ppc/bclwsww     & 1        &  0/0/0/0\\
ppc/lwdwr       & 22       &  0/0/0/0\\
ppc/lwswr       & 4        &  0/0/0/0\\
ppc/podrr       & 4        &  0/0/0/0\\
ppc/podrwposwr  & 16       &  0/0/0/0\\
ppc/podrw       & 2        &  0/0/0/0\\
ppc/podwr       & 2        &  0/0/0/0\\
ppc/podww       & 2        &  0/0/0/0\\
ppc/posrr       & 5        &  0/0/1/1\\
ppc/rfe         & 7        &  0/0/0/0\\
ppc/rfi         & 3        &  0/0/0/0\\
ppc/safe        & 126      &  0/0/0/6\\
ppc/thin        & 8        &  0/0/0/0\\
\bottomrule
\end{tabular}
\caption{Overview of systematic experiments using generated litmus tests \label{tab:litmus-exp}}
\end{table}
